# Supplementary material for: Probabilistic Programming with Gaussian Process Memoization
Source: arXiv:1512.05665 source file (2016-01-05)
Supplement: Supplementary file 2 [file Appendix_SE_kernel.tex]

\myparagraph{Squared-exponential Kernel in Venture}
\begin{lstlisting}[mathescape,escapechar=\#]
assume sf = tag(scope="hyper-parameters", gamma(5,1));
assume l = tag("scope="hyper-parameters", gamma(5,1));
assume kse  = apply_function(make_squaredexp, sf, l);

\end{lstlisting}

\myparagraph{Hierarchical Hyper-priors}
\begin{lstlisting}[mathescape,escapechar=\#]
assume alpha_sf = tag(scope="hyperhyper", gamma(5,1));
assume beta_sf = tag("scope="hyperhyper", gamma(5,1));

assume alpha_l = tag(scope="hyperhyper", gamma(5,1));
assume beta_l = tag("scope="hyperhyper", gamma(5,1));
\end{lstlisting}
